# Supplementary material for: Switching between Magnetic Bloch and N\'eel Domain Walls with Anisotropy Modulations
Source: arXiv:2104.12400 ancillary file (2021-09-09)
Supplement: Supplementary file 1 [file anisotropy_tuning_of_DW_type_SI.pdf]

# Supplemental Information for "Switching between Magnetic Bloch and Néel Domain Walls with Anisotropy Modulations"

Kévin J. A. Franke,[1] Colin Ophus,[2] Andreas K. Schmid,[2] and Christopher H. Marrows[1]

[1]*School of Physics and Astronomy, University of Leeds, Leeds LS2 9JT, United Kingdom*
[2]*National Center for Electron Microscopy, Molecular Foundry, Lawrence Berkeley National Laboratory, Berkeley, California 94720, USA*

(Dated: August 6, 2021)

## I. DMI

Figure S1(a) shows the phase diagram of the DW magnetization angle $\phi$ as a function of $K_{\mathrm{pp}}$ and $D$. It can be contrasted to the one in Fig. 3(a) of the main text showing regions where Bloch and Néel DWs are stabilized as a function of $K_{\mathrm{pp}}$ and $K_{\mathrm{ip}}$. We see that not only is the transition between Bloch and Néel DWs gradual (as opposed to abrupt), but it is also not possible to tune the DW angle with a change in $K_{\mathrm{pp}}$. This is highlighted by the contour lines for DW angles of 15°, 45°, and 75°, that do not show a dependence on $K_{\mathrm{pp}}$. The same can be concluded from Fig. S1(b), where $\phi$ is plotted as a function of $K_{\mathrm{pp}}$ for fixed values of $D$. Again, the curves are completely flat, except at the transition to an in-plane magnetized film. Finally, the dependence of the DW angle on $D$ does not change with $K_{\mathrm{pp}}$, as shown in Fig. S1(c).

## II. COMBINING IN-PLANE ANISOTROPY AND DMI

The phase diagram of the DW magnetization angle $\phi$ as a function of $K_{\mathrm{pp}}$ and $K_{\mathrm{ip}}$ shown in Fig. 3(a) of the main text is distorted by the inclusion of fixed values of $D$ as shown in Fig. S2.

## III. ANALYTICAL MODEL

To understand which type of DW is stabilized as a function of DMI ($D$), and in-plane ($K_{\mathrm{ip}}$) and out-of-plane ($K_{\mathrm{pp}}$) anisotropies we construct a simple one-dimensional analytical model. We look at the dependence of the DW surface energy on the DW magnetization angle $\phi$. The DW surface energy is given by:

$$\sigma_{\mathrm{DW}} = \sigma_{\mathrm{EX}} + \sigma_{\mathrm{K,pp}} + \sigma_{\mathrm{K,ip}} + \sigma_{\mathrm{D,s}} + \sigma_{\mathrm{D,v}} + \sigma_{\mathrm{DMI}}, \quad (1)$$

which is a sum of the exchange energy $\sigma_{\mathrm{EX}}$, perpendicular anisotropy energy $\sigma_{\mathrm{K,pp}}$, in-plane anisotropy energy $\sigma_{\mathrm{K,ip}}$, the demagnetization energy that is here subdivided into the energy associated with (virtual) magnetic surface charges $\sigma_{\mathrm{D,s}}$ and the one associated with (virtual) magnetic volume charges $\sigma_{\mathrm{D,v}}$, and the energy $\sigma_{\mathrm{DMI}}$ due to the DMI.

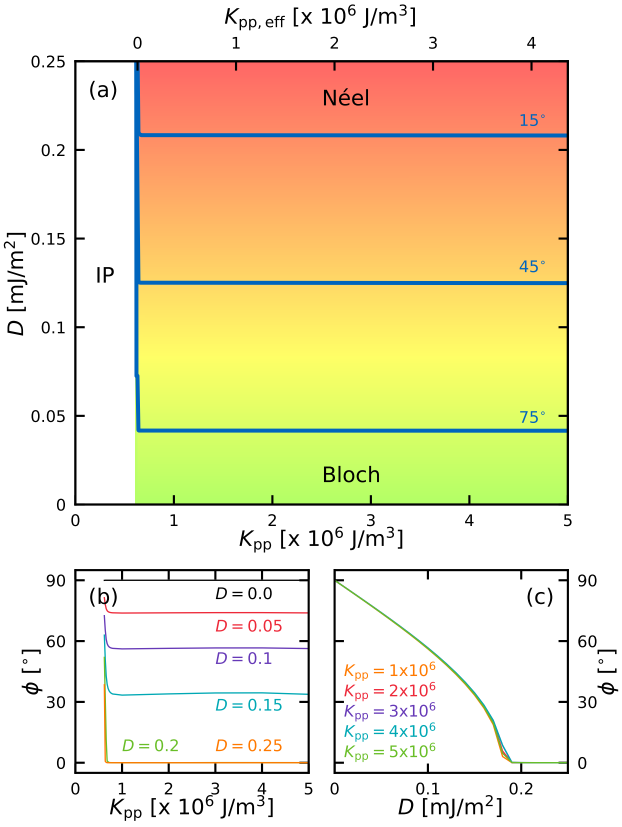


FIG. S1. (a) Phase diagram of the domain wall magnetization angle as a function of $K_{\mathrm{pp}}$ and $D$. (b) Domain wall magnetization angle as a function of $K_{\mathrm{pp}}$ for different values of $D$. (c) Domain wall angle as a function of $D$ for different values of $K_{\mathrm{pp}}$.

We choose the theoretical DW profile centered around $x = 0$ as:[1,2]

$$\vec{m} = \begin{pmatrix} \dfrac{\cos(\phi)}{\cosh(2x/\delta)} \\ \dfrac{\sin(\phi)}{\cosh(2x/\delta)} \\ \tanh(2x/\delta) \end{pmatrix} \quad (2)$$

We compare this theoretical DW profile with the simulated Bloch and Néel domain profiles in Fig. S3, finding very good agreement. The volume charges $\rho_{\mathrm{v}} = -\nabla\vec{m}$ calculated from the DW profiles also show excellent

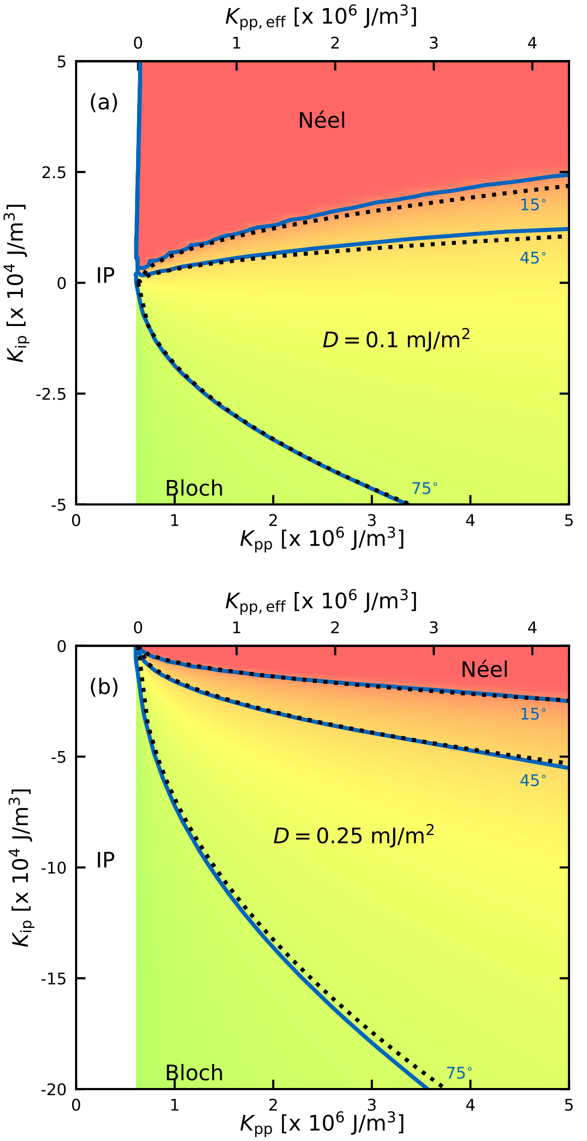


FIG. S2. Phase diagrams of the domain wall magnetization angle as a function of $K_{\rm pp}$ and $K_{\rm ip}$ for fixed values of the DMI constant. (a) $D = 0.1$ mJ/m$^2$ and (b) $D = 0.25$ mJ/m$^2$. Solid blue lines are contour lines of the simulation data for given domain wall angles of 15°, 45°, and 75°. Dotted black lines are the contour lines expected from the analytical model. Note the difference in scale of the $K_{\rm ip}$-axis.

agreement. We thus use this DW profile to compare the energy terms in Eq. 1. We also assume the same DW widths $\delta$ for Bloch and Néel DW. As shown in Fig. 3(c) of the main text, this is a good approximation.

As we are interested in the dependence of the DW surface energy on the DW angle, energy terms that are independent of $\phi$ can be ignored. The exchange surface energy:

$$\sigma_{\rm EX} = \int_{-\infty}^{+\infty} A\,(\nabla\overrightarrow{m})^2 dx = 4\frac{A}{\delta}, \tag{3}$$

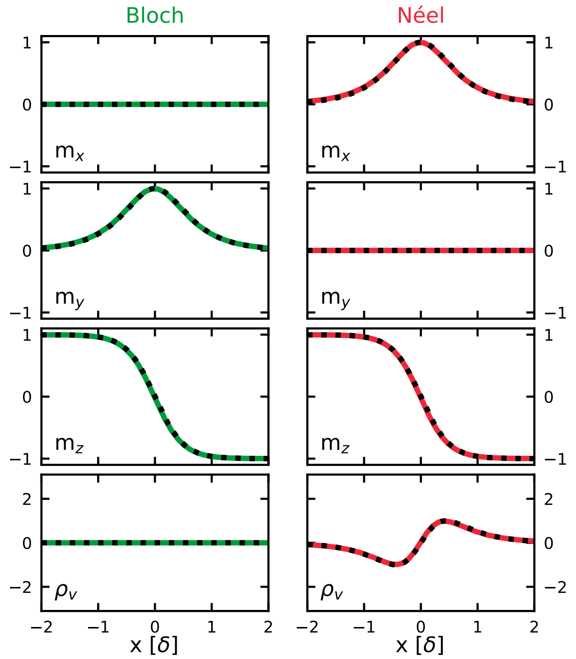


FIG. S3. Profiles of the magnetization components and volume charges of Bloch (left, green) and Néel (right, red) DWs, obtained for $K_{\rm pp} = 1\times10^6$ J/m$^3$, and $K_{\rm ip} = 0$ J/m$^3$ and $K_{\rm ip} = 6\times10^4$ J/m$^3$ for Bloch and Néel DWs, respectively. Black dotted lines show the corresponding profiles obtained from Eq. 2.

depends only on the magnitude of the angle between neighboring spins. It is independent of $\phi$.

The in-plane anisotropy surface energy for an infinitely long DW (along the $y$-axis) in an infinite thin film is given by:

$$\begin{aligned}\sigma_{\rm K,ip} &= \int_{-\infty}^{+\infty} K_{\rm ip}\,\sin^2\psi\,dx \\ &= K_{\rm ip}\int_{-\infty}^{+\infty} 1-(\hat{n}_{\rm ip}\cdot\overrightarrow{m})^2\,dx \\ &= K_{\rm ip}\left(\int_{-\infty}^{+\infty} 1\,dx - \int_{-\infty}^{+\infty}\frac{\cos^2(\phi)}{\cosh^2(2x/\delta)}\,dx\right),\end{aligned} \tag{4}$$

where $\psi$ is the angle between the magnetization and the easy axis of the anisotropy. The first (diverging) integral in the last line of Eq. 4 is independent of the DW angle. It is the in-plane anisotropy energy of the (infinite) domains, and not relevant for the DW energy. The second integral yields the in-plane anisotropy energy of the DW:

$$\sigma_{\rm K,ip} = -K_{\rm ip}\,\delta\,\cos^2(\phi). \tag{5}$$

Similarly the perpendicular anisotropy energy depends on the angle the magnetization makes with the thin film normal $\hat{n}_{\rm pp}$. This means that it depends only on $m_z$, which is independent of $\phi$:[2]

$$\sigma_{\rm K,pp} = \int_{-\infty}^{+\infty} K_{\rm pp}\,(1-m_z^2)\,dx = K_{\rm pp}\,\delta. \tag{6}$$

The demagnetization energy associated with magnetic surface charges $\rho_s = \hat{n}_{pp} \cdot \overrightarrow{m}$ also depends on $m_z$, only, and does not vary with $\phi$. Following Skaugen *et al.* [2], the surface demagnetization energy of the DW associated with volume charges, is given in first order of $(t/\delta)$ by:

$$\sigma_{D,v} = \frac{\ln 2}{\pi}\, \mu_0\, M_s^2\, t\, \cos^2(\phi), \tag{7}$$

for an infinite thin film with constant magnetization in the $z$-direction and thickness $t$ much smaller than relevant magnetic lenght scales, as is the case here. Finally, the DMI energy of the DW is given by:[3]

$$\sigma_{DMI} = -\pi\, D\, \cos(\phi). \tag{8}$$

Hence, only the in-plane anisotropy energy, the magnetostatic energy associated with volume charges, and the DMI energy of the magnetic DW depend on the domain wall magnetization angle. Therefore, taking into account only energy terms that depend on $\phi$, the total DW surface energy is:

$$\sigma(\phi) = \left( \frac{\ln 2}{\pi}\, \mu_0\, M_s^2\, t - K_{ip}\, \delta \right) \cos^2(\phi) - \pi\, D\, \cos(\phi). \tag{9}$$

### A. $D = 0$

In the absence of a DMI ($D = 0$), the difference in DW surface energy between Néel ($\phi = 0°$) and Bloch ($\phi = 90°$) DWs is:

$$\begin{aligned} \Delta\sigma &= \sigma(\phi{=}0°) - \sigma(\phi{=}90°) \\ &= -\frac{\ln 2}{\pi}\, \mu_0\, M_s^2\, t + K_{ip}\, \delta. \end{aligned} \tag{10}$$

The first term yields the magnetostatic energy associated with the formation of a Néel DW. The second term represents the in-plane anisotropy cost of a Bloch DW, due to the fact that the magnetization in the DW is perpendicular to the in-plane easy axis. It depends linearly on the DW width, because the anisotropy energy depends linearly on the number of magnetic moments that are misaligned with the easy axis. As detailed in the main text, the DW width is given by $\delta = 2\sqrt{A/K_{pp,eff}}$. For low $K_{ip}$ values the magnetostatic energy favoring Bloch DWs dominates, while at some point, as $K_{ip}$ increases, the anisotropy energy will dominate, favoring Néel DWs. The transition occurs when $\Delta\sigma = 0$. The in-plane anisotropy constant at which the switch between DW types occurs is thus given by:

$$K_{ip} = \frac{\ln 2\, \mu_0}{2\,\pi} \frac{M_s^2\, t}{\sqrt{A}} \sqrt{K_{pp,eff}}. \tag{11}$$

As shown in Fig. 3(b) of the main text this theoretical value matches results from micromagnetic simulations very well.

### B. $D \neq 0$

For a finite DMI, we can use the analytical model to reproduce the contour lines in Fig. 5 of the main text and Fig. S2 of the Supplemental Information. Setting the partial derivative of the DW surface energy in Eq. 9 with respect to $\phi$ to zero, we find that the DW surface energy is minimized when:

$$K_{ip} = \frac{\ln 2\, \mu_0}{2\,\pi} \frac{M_s^2\, t}{\sqrt{A}} \sqrt{K_{pp,eff}} - \frac{\pi}{4\sqrt{A}} \sqrt{K_{pp,eff}}\, \frac{D}{\cos\phi}. \tag{12}$$

We see, that the contour lines for a given $\phi$ and $K_{pp}$ are linear in $-D$. They are compared to the results from micromagnetic simulations in Fig. 5 of the main text, where we observe excellent agreement. We also see that the contour lines for a given $\phi$ and $K_{ip}$ are expected to be proportional to $\sqrt{K_{pp,eff}}$. This is superimposed in Fig. S2 of the Supplemental Information, again demonstrating good agreement with micromagnetic simulations.

### C. Nanowire Geometry

The phase diagram in Fig. 4 of the main text for a nanowire geometry can be understood in terms of the analytical model for the thin film geometry when the demagnetization energy is expressed as an effective anisotropy. For a uniformly magnetized nanowire, the demagnetization energy density is given by:

$$e_D = \frac{1}{2}\, \mu_0\, \left( N_x M_x^2 + N_z M_z^2 \right), \tag{13}$$

where $M_i$ are the magnetization components, and $N_i$ are the demagnetizing factors with $N_x + N_z = 1$.[4] Following Brown [5],

$$N_z = \frac{2}{\pi}\arctan\left(\frac{1}{p}\right) + \frac{p}{\pi}\ln(p) + \left(\frac{1-p^2}{2\pi p}\right)\ln\left(1+p^2\right) \tag{14}$$

where $p = t/w$ is the ratio between the nanowire thickness $t$ and width $w$. The effective anisotropy constants can then be written as:

$$K_{ip,eff} = K_{ip} + \frac{1}{2}\, \mu_0\, N_x M_x^2, \tag{15}$$

and

$$K_{pp,eff} = K_{pp} - \frac{1}{2}\, \mu_0\, N_z M_z^2. \tag{16}$$

## IV. DOMAIN WALL WIDTHS

The DW widths $\delta$ obtained from micromagnetic simulations as a function of $D$ and $K_{ip}$ for $K_{pp} = 1{\times}10^6$ J/m$^3$ are shown in Fig. S4. The corresponding DW magnetization angles $\phi$ are shown in Figs. 2(d) & (e) of the main

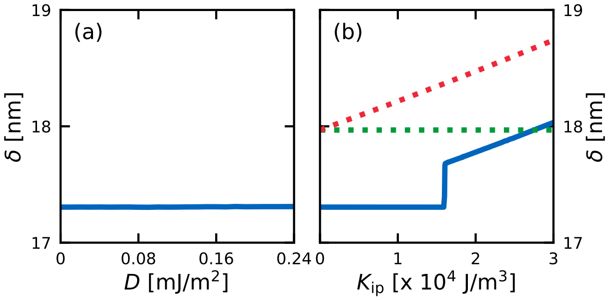


FIG. S4. DW widths $\delta$ obtained from micromagnetic simulations (blue lines) as a function of (a) $D$ and (b) $K_{\rm ip}$ for $K_{\rm pp} = 1{\times}10^6$ J/m$^3$. Corresponding analytical DW widths for Bloch (green dotted) and Néel (red dotted) DWs as a function of $K_{\rm ip}$.

manuscript. The DW width does not depend on $D$ and is thus independent of the type of DW that is stabilised. On the other hand, when an in-plane anisotropy is used to switch between DW types the width is affected by $K_{\rm ip}$. While the width of Bloch DWs does not seem affected by $K_{\rm ip}$, a jump in $\delta$ is observed as the type of DW switches to Néel. Subsequently, the DW width increases with the in-plane anisotropy strength.

An analytical expression for $\delta$ can be obtained by setting the partial derivative of the surface energy with respect to $\delta$ equal to zero. Taking into account only terms that depend on $\delta$, the DW surface energy is:

$$\begin{aligned}\sigma(\delta) &= \sigma_{\rm EX} + \sigma_{\rm K,pp,eff} + \sigma_{\rm K,ip} \\ &= 4\frac{A}{\delta} + K_{\rm pp,eff}\,\delta - K_{\rm ip}\,\delta\,\cos^2(\phi),\end{aligned} \tag{17}$$

where we have taken the effect of the demagnetization energy associated with magnetic surface charges into account in the effective perpendicular magnetic anisotropy. Setting the partial derivative with respect to $\delta$ equal to zero and solving for the DW width, one obtains:

$$\delta = 2\sqrt{\frac{A}{K_{\rm pp,eff} - K_{\rm ip}\cos^2(\phi)}}. \tag{18}$$

From this expression we expect that $\delta$ does not depend on $D$, as seen in Fig. S4(a). Is is also independed of $K_{\rm ip}$ for Bloch DWs ($\phi = \pm 90°$). For Néel DWs $\delta$ is predicted to increase with increasing $K_{\rm ip}$. The analytical DW widths for Bloch (green dotted) and Néel (red dotted) DWs as a function of $K_{\rm ip}$ are compared to the results from micromagnetic simulations in Fig. S4(b). They show excellent qualitative agreement. The small quantitative difference of $\approx 5\%$ is exagerated by the choise of scale on the $\delta$-axis. The jump in $\delta$ at the transition between Bloch and Néel DWs is even smaller, due to the fact that $K_{\rm ip}$ is two orders of magnitude smaller than $K_{\rm pp}$. It is therefore reasonable to approximate the DW width as $\delta = 2\sqrt{A/K_{\rm pp,eff}}$ in the analytical determination of the location of the switch between DW types.

[1] A. Hubert and R. Schäfer, *Magnetic domains: the analysis of magnetic microstructures* (Springer, 1998).

[2] A. Skaugen, P. Murray, and L. Laurson, Phys. Rev. B **100**, 094440 (2019).

[3] A. Thiaville, S. Rohart, É. Jué, V. Cros, and A. Fert, EPL **100**, 57002 (2012).

[4] M. D. DeJong and K. L. Livesey, Phys. Rev. B **92**, 214420 (2015).

[5] W. Brown, *Magnetostatic Principles in Ferromagnetism*, Selected topics in solid state physics (North-Holland Publishing Company, 1962).
